# Supplementary material for: Distinguishability Investigation on Longa's Atomic Patterns when used as a Basis for Implementing Elliptic Curve Scalar Multiplication Algorithms
Source: arXiv:2409.13742 source file (2024-09-10)
Supplement: Supplementary file 1 [file Appendix3.tex]

% Appendix

\section{Study of FLECC Field Operations} % Main appendix title

\label{Appendix3}

For those who are interested in the implementation of constant-time field operation functions using FLECC, we measured the execution time of those we used in Doubling 2 of our atomic patterns algorithm using software breakpoints in CCS with the code executed in RAM. As shown in Table \ref{flecc_exe_time}, the execution time of each operation was measured in number of clock cycles and then converted into time in millisecond according to our experimental equipment configurations. 

\begin{table}[H]
\centering
\begin{tabular}{|l|c|c|}
\hline
               & No. of clock cycles & Time($ms$) \\ \hline
$1^{st}$ Multiplication (X) & 16570            &     0.166     \\ \hline
$2^{nd}$ Multiplication (X') & 16569            &     0.166     \\ \hline
Negation (N)       & 1197            &     0.0120     \\ \hline
Addition (A)       & 1353            &     0.0135     \\ \hline
\end{tabular}\caption{Execution time of FLECC field operations in Doubling 2 $\Delta1$.}\label{flecc_exe_time}
\end{table}

Although the execution time might deviate in practice when the code is executed on hardware, we used this software execution time information to estimate the duration of each atomic pattern in our measured traces. In Figure \ref{fig:1st_atom_pattern}, based on Figure \ref{atom1_syncB}, we marked the areas of the atomic block's sub-trace in white fonts and dashed lines to indicate the execution time of each mathematical operation according to their software execution time. Moreover, we observed that FLECC's Montgomery modular multiplication operation does not have constant runtime (see Table \ref{flecc_exe_time}).

\begin{figure}[H]
\centering
\includegraphics[width=1\textwidth]{Figures/1st_atom_pattern.png}
\caption{Estimated atomic patterns distribution in $\Delta1$.}
\label{fig:1st_atom_pattern}
\end{figure}

\begin{table}[!ht]
    \centering
    \begin{tabular}{|l|l|l|l|}
    \hline
        X & Start & End & Duration  \\ \hline
        Doubling 1 & 533427 & 549992 & 16565 \\ \hline
        Doubling 2 & 1052586 & 1069156 & 16570  \\ \hline
        Doubling 3 & 1571720 & 1588285 & 16565  \\ \hline
        Doubling 4 & 2673531 & 2690101 & 16570  \\ \hline
        Doubling 5 & 3775323 & 3791893 & 16570  \\ \hline
        Doubling 6 & 4294499 & 4311069 & 16570  \\ \hline
        Doubling 7 & 5396316 & 5412881 & 16565  \\ \hline
        Doubling 8 & 6498128 & 6514693 & 16565  \\ \hline
        Doubling 9 & 7017274 & 7033839 & 16565  \\ \hline
        Doubling 10 & 8119076 & 8135641 & 16565  \\ \hline
        Doubling 11 & 8638222 & 8654787 & 16565  \\ \hline
        Doubling 12 & 9740014 & 9756579 & 16565  \\ \hline
        Doubling 13 & 10841816 & 10858381 & 16565  \\ \hline
        Doubling 14 & 11943608 & 11960178 & 16570  \\ \hline
        Doubling 15 & 13045420 & 13061990 & 16570  \\ \hline
        Doubling 16 & 14147227 & 14163797 & 16570  \\ \hline
        Doubling 17 & 15249054 & 15265619 & 16565  \\ \hline
        Doubling 18 & 16350836 & 16367406 & 16570  \\ \hline
        Doubling 19 & 16870007 & 16886572 & 16565  \\ \hline
        Doubling 20 & 17971794 & 17988359 & 16565  \\ \hline
        Doubling 21 & 19073625 & 19090190 & 16565  \\ \hline \hhline{|=|=|=|=|}
        Addition 1 & 2020871 & 2037436 & 16565  \\ \hline
        Addition 2 & 3122673 & 3139238 & 16565  \\ \hline
        Addition 3 & 4743655 & 4760225 & 16570  \\ \hline
        Addition 4 & 5845472 & 5862037 & 16565  \\ \hline
        Addition 5 & 7466429 & 7482994 & 16565  \\ \hline
        Addition 6 & 9087376 & 9103941 & 16565  \\ \hline
        Addition 7 & 10189168 & 10205733 & 16565  \\ \hline
        Addition 8 & 11290970 & 11307535 & 16565  \\ \hline
        Addition 9 & 12392772 & 12409337 & 16565  \\ \hline
        Addition 10 & 13494584 & 13511149 & 16565  \\ \hline
        Addition 11 & 14596411 & 14612976 & 16565  \\ \hline
        Addition 12 & 15698193 & 15714758 & 16565  \\ \hline
        Addition 13 & 17319150 & 17335715 & 16565  \\ \hline
        Addition 14 & 18420947 & 18437512 & 16565  \\ \hline
        Addition 15 & 19522734 & 19539299 & 16565 \\ \hline
    \end{tabular}
    \caption{Execution time of the first X operation in $\Delta1$ of each point operation, measured in clock cycles.}\label{x_exec_time}
\end{table}
